# Supplementary material for: CaLDiff: Camera Localization in NeRF via Pose Diffusion
Source: arXiv:2312.15242 source file (2023-12-23)
Supplement: Supplementary file 1 [file supp.tex]

\begin{table*}[]
\centering
\begin{tabular}{ll}
\begin{tabular}{ccc}

% GT image & CaLDiff Render & Error Map \\

\multicolumn{3}{c}{\textbf{chess}} \\

\vspace{-0.3em}
\includegraphics[width=\iw]{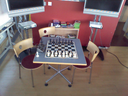} & 
\includegraphics[width=\iw]{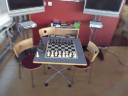} & 
\includegraphics[width=\iw]{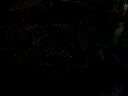} \\

\vspace{0.5em}
& (0.0081, 0.51) & \\

\vspace{-0.3em}
\includegraphics[width=\iw]{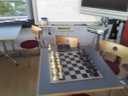} & 
\includegraphics[width=\iw]{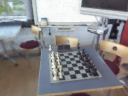} & 
\includegraphics[width=\iw]{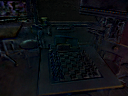} \\

\vspace{0.5em}
& (0.0270, 2.78) & \\

\vspace{-0.3em}
\includegraphics[width=\iw]{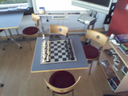} & 
\includegraphics[width=\iw]{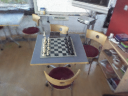} & 
\includegraphics[width=\iw]{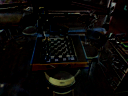} \\

\vspace{0.5em}
& (0.0605, 5.52) & \\

\vspace{-0.3em}
\includegraphics[width=\iw]{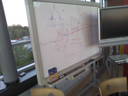} & 
\includegraphics[width=\iw]{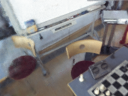} & 
\includegraphics[width=\iw]{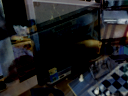} \\

\vspace{0.5em}
& (0.2058, 37.11) & \\

% \hline \\
% \vspace{1em}
% \includegraphics[width=\iw]{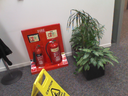} & 
% \includegraphics[width=\iw]{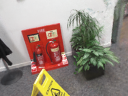} & 
% \includegraphics[width=\iw]{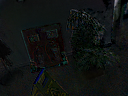} \\

\end{tabular} & \begin{tabular}{ccc}

% GT image & CaLDiff Render & Error Map \\

\multicolumn{3}{c}{\textbf{fire}} \\

\vspace{-0.3em}
\includegraphics[width=\iw]{supp-images/fire/seq-03-frame-000000.color.png--gt.png} & 
\includegraphics[width=\iw]{supp-images/fire/seq-03-frame-000000.color.png-render.png} & 
\includegraphics[width=\iw]{supp-images/fire/seq-03-frame-000000.color.png--diff.png} \\

\vspace{0.5em}
& (0.0057, 1.04) & \\

\vspace{-0.3em}
\includegraphics[width=\iw]{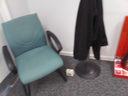} & 
\includegraphics[width=\iw]{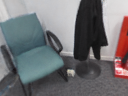} & 
\includegraphics[width=\iw]{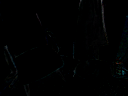} \\

\vspace{0.5em}
& (0.0117, 2.69) & \\

\vspace{-0.3em}
\includegraphics[width=\iw]{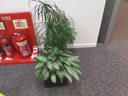} & 
\includegraphics[width=\iw]{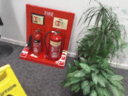} & 
\includegraphics[width=\iw]{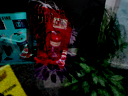} \\

\vspace{0.5em}
& (0.1100, 18.33) & \\

\vspace{-0.3em}
\includegraphics[width=\iw]{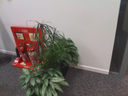} & 
\includegraphics[width=\iw]{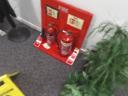} & 
\includegraphics[width=\iw]{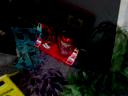} \\

\vspace{0.5em}
& (0.2789, 27.08) & \\

% \hline \\
% \vspace{1em}
% \includegraphics[width=\iw]{supp-images/fire/seq-03-frame-000000.color.png--gt.png} & 
% \includegraphics[width=\iw]{supp-images/fire/seq-03-frame-000000.color.png-render.png} & 
% \includegraphics[width=\iw]{supp-images/fire/seq-03-frame-000000.color.png--diff.png} \\

\end{tabular} \\
\begin{tabular}{ccc}

% GT image & CaLDiff Render & Error Map \\

\multicolumn{3}{c}{\textbf{heads}} \\

\vspace{-0.3em}
\includegraphics[width=\iw]{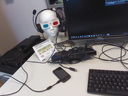} & 
\includegraphics[width=\iw]{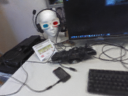} & 
\includegraphics[width=\iw]{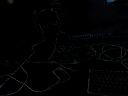} \\

\vspace{0.5em}
& (0.0023, 0.349) & \\

\vspace{-0.3em}
\includegraphics[width=\iw]{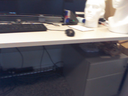} & 
\includegraphics[width=\iw]{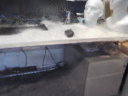} & 
\includegraphics[width=\iw]{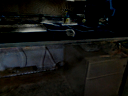} \\

\vspace{0.5em}
& (0.0304, 2.44) & \\

\vspace{-0.3em}
\includegraphics[width=\iw]{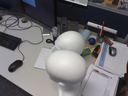} & 
\includegraphics[width=\iw]{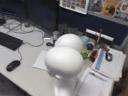} & 
\includegraphics[width=\iw]{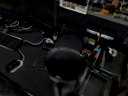} \\

\vspace{0.5em}
& (0.0443, 7.78) & \\

\vspace{-0.3em}
\includegraphics[width=\iw]{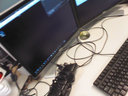} & 
\includegraphics[width=\iw]{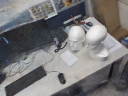} & 
\includegraphics[width=\iw]{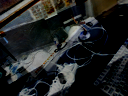} \\

\vspace{0.5em}
& (0.5316, 19.38) & \\

% \hline \\
% \vspace{1em}
% \includegraphics[width=\iw]{supp-images/fire/seq-03-frame-000000.color.png--gt.png} & 
% \includegraphics[width=\iw]{supp-images/fire/seq-03-frame-000000.color.png-render.png} & 
% \includegraphics[width=\iw]{supp-images/fire/seq-03-frame-000000.color.png--diff.png} \\

\end{tabular} &  \begin{tabular}{ccc}

% GT image & CaLDiff Render & Error Map \\

\multicolumn{3}{c}{\textbf{stairs}} \\

\vspace{-0.3em}
\includegraphics[width=\iw]{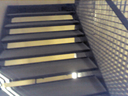} & 
\includegraphics[width=\iw]{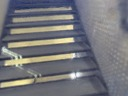} & 
\includegraphics[width=\iw]{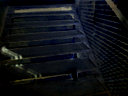} \\

\vspace{0.5em}
& (0.0766, 1.53) & \\

\vspace{-0.3em}
\includegraphics[width=\iw]{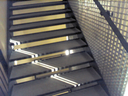} & 
\includegraphics[width=\iw]{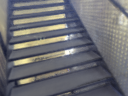} & 
\includegraphics[width=\iw]{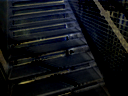} \\

\vspace{0.5em}
& (0.1011, 3.27) & \\

\vspace{-0.3em}
\includegraphics[width=\iw]{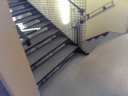} & 
\includegraphics[width=\iw]{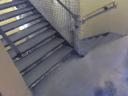} & 
\includegraphics[width=\iw]{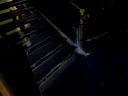} \\

\vspace{0.5em}
& (0.1015, 7.80) & \\

\vspace{-0.3em}
\includegraphics[width=\iw]{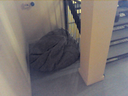} & 
\includegraphics[width=\iw]{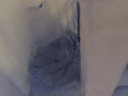} & 
\includegraphics[width=\iw]{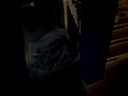} \\

\vspace{0.5em}
& (0.1791, 16.84) & \\

% \hline \\
% \vspace{1em}
% \includegraphics[width=\iw]{supp-images/fire/seq-03-frame-000000.color.png--gt.png} & 
% \includegraphics[width=\iw]{supp-images/fire/seq-03-frame-000000.color.png-render.png} & 
% \includegraphics[width=\iw]{supp-images/fire/seq-03-frame-000000.color.png--diff.png} \\

\end{tabular} \\
\end{tabular}
\caption{Comparison of images rendered with CaLDiff poses and the corresponding ground-truth images for the scenes chess, fire, heads, stairs of 7scenes dataset. For each scene, we present ground-truth image (left), rendered image (middle), and error map (right). We present poses that fall in 4 thresholds: (0.01,2°), (0.025,5°), (0.05,10°), and (0.1,20°) starting from top to bottom.}
\end{table*}

\begin{table*}[]
\centering
\begin{tabular}{ll}
\begin{tabular}{ccc}

% GT image & CaLDiff Render & Error Map \\

\multicolumn{3}{c}{\textbf{room1}} \\

% \vspace{-0.3em}
\includegraphics[width=\iw,angle=-90,origin=c]{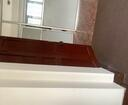} & 
\includegraphics[width=\iw,angle=-90,origin=c]{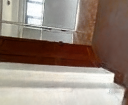} & 
\includegraphics[width=\iw,angle=-90,origin=c]{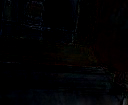} \\

\vspace{0.5em}
& (0.0064, 0.42) & \\

% \vspace{-0.3em}
\includegraphics[width=\iw,angle=-90,origin=c]{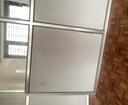} & 
\includegraphics[width=\iw,angle=-90,origin=c]{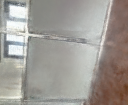} & 
\includegraphics[width=\iw,angle=-90,origin=c]{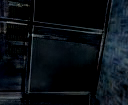} \\

\vspace{0.5em}
& (0.0604, 4.25) & \\

% \vspace{-0.3em}
\includegraphics[width=\iw,angle=-90,origin=c]{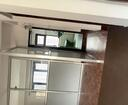} & 
\includegraphics[width=\iw,angle=-90,origin=c]{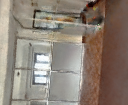} & 
\includegraphics[width=\iw,angle=-90,origin=c]{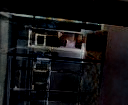} \\

\vspace{0.5em}
& (0.2731, 8.19) & \\

% \vspace{-0.3em}
\includegraphics[width=\iw,angle=-90,origin=c]{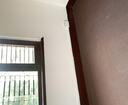} & 
\includegraphics[width=\iw,angle=-90,origin=c]{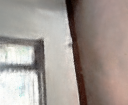} & 
\includegraphics[width=\iw,angle=-90,origin=c]{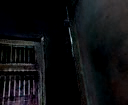} \\

\vspace{0.5em}
& (0.1687, 93.11) & \\

\end{tabular} & \begin{tabular}{ccc}

% GT image & CaLDiff Render & Error Map \\

\multicolumn{3}{c}{\textbf{room2}} \\

% \vspace{-0.3em}
\includegraphics[width=\iw,angle=-90,origin=c]{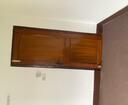} & 
\includegraphics[width=\iw,angle=-90,origin=c]{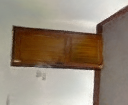} & 
\includegraphics[width=\iw,angle=-90,origin=c]{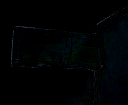} \\

\vspace{0.5em}
& (0.0359, 0.53) & \\

% \vspace{-0.3em}
\includegraphics[width=\iw,angle=-90,origin=c]{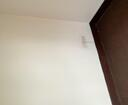} & 
\includegraphics[width=\iw,angle=-90,origin=c]{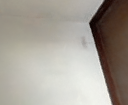} & 
\includegraphics[width=\iw,angle=-90,origin=c]{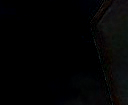} \\

\vspace{0.5em}
& (0.0305, 2.52) & \\

% \vspace{-0.3em}
\includegraphics[width=\iw,angle=-90,origin=c]{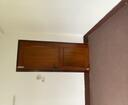} & 
\includegraphics[width=\iw,angle=-90,origin=c]{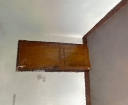} & 
\includegraphics[width=\iw,angle=-90,origin=c]{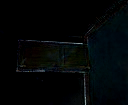} \\

\vspace{0.5em}
& (0.0849, 5.3) & \\

% \vspace{-0.3em}
\includegraphics[width=\iw,angle=-90,origin=c]{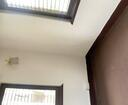} & 
\includegraphics[width=\iw,angle=-90,origin=c]{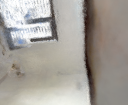} & 
\includegraphics[width=\iw,angle=-90,origin=c]{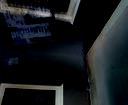} \\

\vspace{0.5em}
& (0.3288, 57.34) & \\

\end{tabular} \\
\begin{tabular}{ccc}

% GT image & CaLDiff Render & Error Map \\

\multicolumn{3}{c}{\textbf{room5}} \\

% \vspace{-0.3em}
\includegraphics[width=\iw,angle=-90,origin=c]{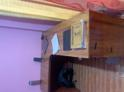} & 
\includegraphics[width=\iw,angle=-90,origin=c]{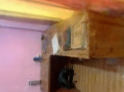} & 
\includegraphics[width=\iw,angle=-90,origin=c]{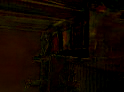} \\

\vspace{0.5em}
& (0.0025, 0.06) & \\

% \vspace{-0.3em}
\includegraphics[width=\iw,angle=-90,origin=c]{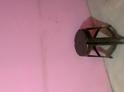} & 
\includegraphics[width=\iw,angle=-90,origin=c]{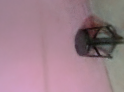} & 
\includegraphics[width=\iw,angle=-90,origin=c]{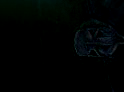} \\

\vspace{0.5em}
& (0.0163, 2.88) & \\

% \vspace{-0.3em}
\includegraphics[width=\iw,angle=-90,origin=c]{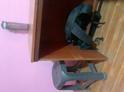} & 
\includegraphics[width=\iw,angle=-90,origin=c]{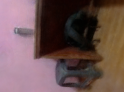} & 
\includegraphics[width=\iw,angle=-90,origin=c]{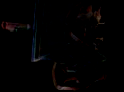} \\

\vspace{0.5em}
& (0.0590, 8.20) & \\

% \vspace{-0.3em}
\includegraphics[width=\iw,angle=-90,origin=c]{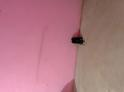} & 
\includegraphics[width=\iw,angle=-90,origin=c]{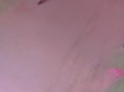} & 
\includegraphics[width=\iw,angle=-90,origin=c]{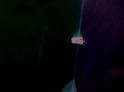} \\

\vspace{0.5em}
& (0.2801, 41.00) & \\

\end{tabular} &  \begin{tabular}{ccc}

% GT image & CaLDiff Render & Error Map \\

\multicolumn{3}{c}{\textbf{stairs1}} \\

% \vspace{-0.3em}
\includegraphics[width=\iw,angle=-90,origin=c]{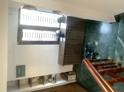} & 
\includegraphics[width=\iw,angle=-90,origin=c]{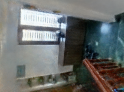} & 
\includegraphics[width=\iw,angle=-90,origin=c]{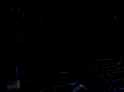} \\

\vspace{0.5em}
& (0.0034, 0.51) & \\

% \vspace{-0.3em}
\includegraphics[width=\iw,angle=-90,origin=c]{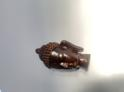} & 
\includegraphics[width=\iw,angle=-90,origin=c]{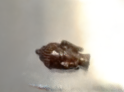} & 
\includegraphics[width=\iw,angle=-90,origin=c]{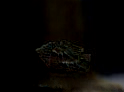} \\

\vspace{0.5em}
& (0.0122, 4.44) & \\

% \vspace{-0.3em}
\includegraphics[width=\iw,angle=-90,origin=c]{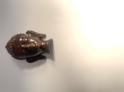} & 
\includegraphics[width=\iw,angle=-90,origin=c]{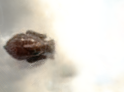} & 
\includegraphics[width=\iw,angle=-90,origin=c]{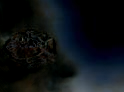} \\

\vspace{0.5em}
& (0.0194, 7.26) & \\

% \vspace{-0.3em}
\includegraphics[width=\iw,angle=-90,origin=c]{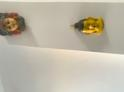} & 
\includegraphics[width=\iw,angle=-90,origin=c]{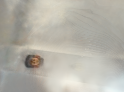} & 
\includegraphics[width=\iw,angle=-90,origin=c]{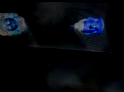} \\

\vspace{0.5em}
& (0.1098, 29.21) & \\

\end{tabular} \\
\end{tabular}
\caption{Comparison of images rendered with CaLDiff poses and the corresponding ground-truth images for the scenes room1, room2, room5, stairs1 of Empty rooms dataset.}
\end{table*}

\begin{table*}[]
\centering
\begin{tabular}{ll}
\begin{tabular}{ccc}

% GT image & CaLDiff Render & Error Map \\

\multicolumn{3}{c}{\textbf{room3}} \\

% \vspace{-0.3em}
\includegraphics[width=\iw,angle=-90,origin=c]{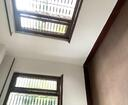} & 
\includegraphics[width=\iw,angle=-90,origin=c]{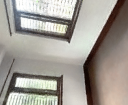} & 
\includegraphics[width=\iw,angle=-90,origin=c]{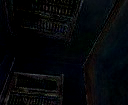} \\

\vspace{0.5em}
& (0.0100, 0.80) & \\

% \vspace{-0.3em}
\includegraphics[width=\iw,angle=-90,origin=c]{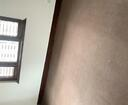} & 
\includegraphics[width=\iw,angle=-90,origin=c]{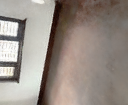} & 
\includegraphics[width=\iw,angle=-90,origin=c]{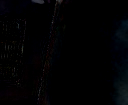} \\

\vspace{0.5em}
& (0.0258, 2.04) & \\

% \vspace{-0.3em}
\includegraphics[width=\iw,angle=-90,origin=c]{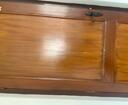} & 
\includegraphics[width=\iw,angle=-90,origin=c]{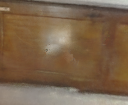} & 
\includegraphics[width=\iw,angle=-90,origin=c]{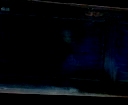} \\

\vspace{0.5em}
& (0.0319, 6.98) & \\

% \vspace{-0.3em}
\includegraphics[width=\iw,angle=-90,origin=c]{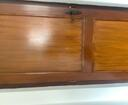} & 
\includegraphics[width=\iw,angle=-90,origin=c]{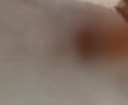} & 
\includegraphics[width=\iw,angle=-90,origin=c]{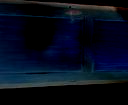} \\

\vspace{0.5em}
& (0.0625, 55.83) & \\

\end{tabular} & \begin{tabular}{ccc}

% GT image & CaLDiff Render & Error Map \\

\multicolumn{3}{c}{\textbf{room4}} \\

% \vspace{-0.3em}
\includegraphics[width=\iw,angle=-90,origin=c]{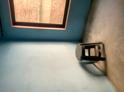} & 
\includegraphics[width=\iw,angle=-90,origin=c]{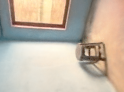} & 
\includegraphics[width=\iw,angle=-90,origin=c]{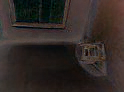} \\

\vspace{0.5em}
& (0.0193, 1.56) & \\

% \vspace{-0.3em}
\includegraphics[width=\iw,angle=-90,origin=c]{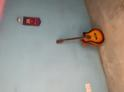} & 
\includegraphics[width=\iw,angle=-90,origin=c]{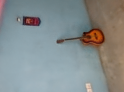} & 
\includegraphics[width=\iw,angle=-90,origin=c]{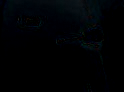} \\

\vspace{0.5em}
& (0.0254, 2.25) & \\

% \vspace{-0.3em}
\includegraphics[width=\iw,angle=-90,origin=c]{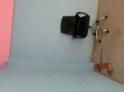} & 
\includegraphics[width=\iw,angle=-90,origin=c]{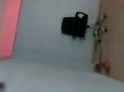} & 
\includegraphics[width=\iw,angle=-90,origin=c]{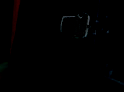} \\

\vspace{0.5em}
& (0.1231, 9.97) & \\

% \vspace{-0.3em}
\includegraphics[width=\iw,angle=-90,origin=c]{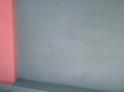} & 
\includegraphics[width=\iw,angle=-90,origin=c]{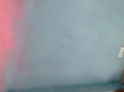} & 
\includegraphics[width=\iw,angle=-90,origin=c]{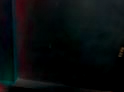} \\

\vspace{0.5em}
& (0.3215, 42.85) & \\

\end{tabular} \\
\begin{tabular}{ccc}

% GT image & CaLDiff Render & Error Map \\

\multicolumn{3}{c}{\textbf{room6}} \\

% \vspace{-0.3em}
\includegraphics[width=\iw,angle=-90,origin=c]{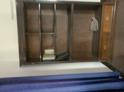} & 
\includegraphics[width=\iw,angle=-90,origin=c]{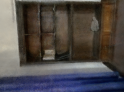} & 
\includegraphics[width=\iw,angle=-90,origin=c]{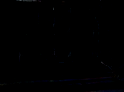} \\

\vspace{0.5em}
& (0.0185, 1.83) & \\

% \vspace{-0.3em}
\includegraphics[width=\iw,angle=-90,origin=c]{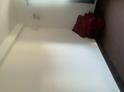} & 
\includegraphics[width=\iw,angle=-90,origin=c]{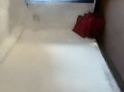} & 
\includegraphics[width=\iw,angle=-90,origin=c]{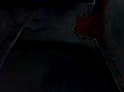} \\

\vspace{0.5em}
& (0.0162, 2.14) & \\

% \vspace{-0.3em}
\includegraphics[width=\iw,angle=-90,origin=c]{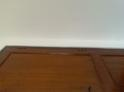} & 
\includegraphics[width=\iw,angle=-90,origin=c]{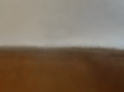} & 
\includegraphics[width=\iw,angle=-90,origin=c]{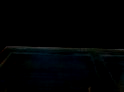} \\

\vspace{0.5em}
& (0.1326, 14.67) & \\

% \vspace{-0.3em}
\includegraphics[width=\iw,angle=-90,origin=c]{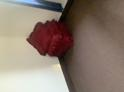} & 
\includegraphics[width=\iw,angle=-90,origin=c]{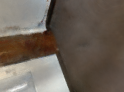} & 
\includegraphics[width=\iw,angle=-90,origin=c]{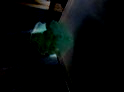} \\

\vspace{0.5em}
& (0.1090, 99.17) & \\

\end{tabular} & \\
\end{tabular}
\caption{Comparison of images rendered with CaLDiff poses and the corresponding ground-truth images for the scenes room3, room4, room6 of Empty rooms dataset.}
\end{table*}
